# Supplementary material for: Wild ToFu: Improving Range and Quality of Indirect Time-of-Flight Depth with RGB Fusion in Challenging Environments
Source: arXiv:2112.03750 source file (2022-06-16)
Supplement: Supplementary file 1 [file _supplimentary_abliation_figures.tex]

\section{Ablation study figures} \label{sec:supplimentary_ablation}

\subsection{1/4 res bottleneck VS 1/32 res bottleneck}

\paragraph{without Fusion}

\begin{figure}[htpb]
    \centering
    \includegraphics[width=\linewidth]{images/1_32_vs_1_4_no_fusuion.PNG}
    \caption{Improvement with 1/32 resolution bottleneck without fusion.}
    \label{fig:1_4_vs_1_32_improvement}
\end{figure}

Fig.\ref{fig:1_4_vs_1_32_improvement} shows improvement by using architecture with 1/32 resolution bottleneck (MD2 \cite{monodepth2})compared to 1/4 resolution bottleneck (ToFNet \cite{su}) due to better global context extraction. Most of quantitative improvement is result of resolving phase unwrapping problem with better global context cue.

\paragraph{with Fusion}

\subsection{Implicitly aligned fusion VS Attention fusion}

\subsection{Bottleneck fusion VS All resolution fusion}
