# Supplementary material for: Wild ToFu: Improving Range and Quality of Indirect Time-of-Flight Depth with RGB Fusion in Challenging Environments
Source: arXiv:2112.03750 source file (2022-06-16)
Supplement: Supplementary file 2 [file _supplimentary_architecture.tex]

\section{Detailed architecture} \label{sec:supplimentary_architecture}
